# Supplementary material for: Impact of Perturbations on Watersheds
Source: arXiv:1101.5890 source file (2011-01-31)
Supplement: Supplementary file 1 [file supplement.pdf]

# Online Supplementary Materials

In Fig. SM1 we show the distribution $P(R)$ for natural landscapes of various regions, namely, Rocky Mountains, Andes and Appalachian (unshifted); Brazil and Europe (shifted by a factor of 100 for better visibility); US-CAN, Kongo and Germany (shifted by a factor of 10000). All data sets have a resolution of 540 m. The solid line shows the best fit to the Andes data with a power-law of exponent $-3.1 \pm 0.3$. The inset of Fig. SM1 shows the corresponding distributions $P(A|R)$ associated with the outlet distance $R = 0.54$ km. The solid line is the best fit of a power-law to the Andes data with an exponent $-2.3 \pm 0.2$.

As shown in Fig. SM2, the enclosed areas for uncorrelated landscapes are indeed compact. Here, the average area $\langle A \rangle$ is presented as a function of the outlet distance $R$ for different system sizes. Considering finite-size scaling, our data is consistent with $< A > \propto R^2$, as depicted by the solid line with slope 2. The inset of Fig. SM2 shows the data collapse of the distribution $P(A|R)$ associated with an outlet distance $R = 1, 10$ (filled and open symbols, respectively) for different system sizes. The solid lines are the best fits to the data of a power-law with an exponent $-2.23 \pm 0.03$.

Finally, we show in Fig. SM3 the data collapse of the distribution $P(M|R)$ associated with outlet distances $R = 1$ and 10 (filled and open symbols, respectively) for three different system sizes. The two solid lines correspond to power-laws with an exponent $(\alpha^* + 1) = 2.39$, where $\alpha^*$ corresponds to the exponent for subcritical point-to-point invasion percolation model.

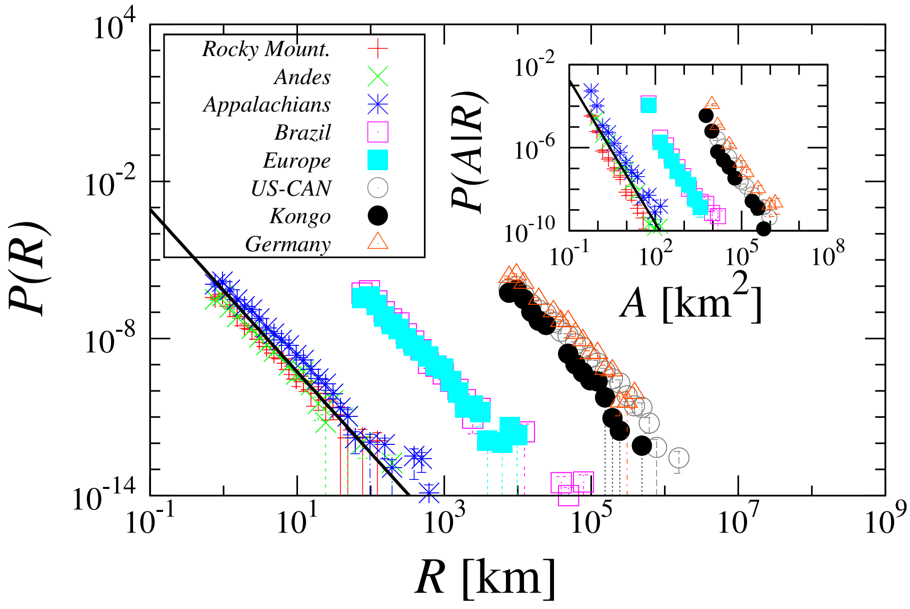


Figure SM1: (color online) Distribution of outlet distances $R$ for various natural landscapes. The solid line is the best fit to the data of the power-law, $P(R) \propto R^{-\rho}$, with $\rho = 3.1 \pm 0.3$. The inset shows the distributions $P(A|R)$ associated with the outlet distance $R = 0.54$ km. The solid line is the best fit to the Andes data of the power-law, $P(A|R) \propto R^{-\alpha}$, with $\alpha = 2.3 \pm 0.2$.

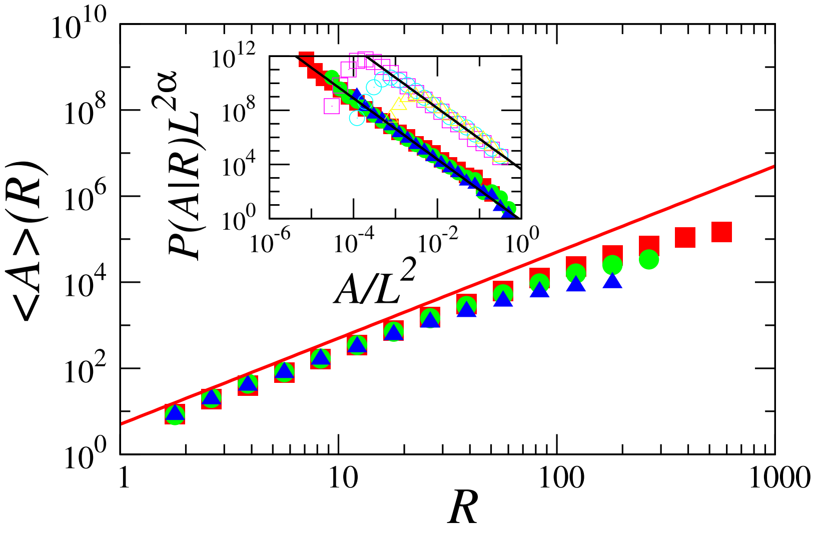


Figure SM2: (color online) Dependence of the average area $\langle A \rangle$ on the outlet distance $R$ for different sizes of uncorrelated landscapes, namely, $L = 129, 257, 513$ (triangles, circles, square, respectively). The solid line has slope 2. The inset shows the data collapse of $P(A|R)$ for $R = 1$ and 10 (filled and open symbols, respectively), and the same system sizes. The solid lines correspond to power-laws, $P(A|R) \propto R^{-\alpha}$, with the same exponent $\alpha = 2.23 \pm 0.03$.

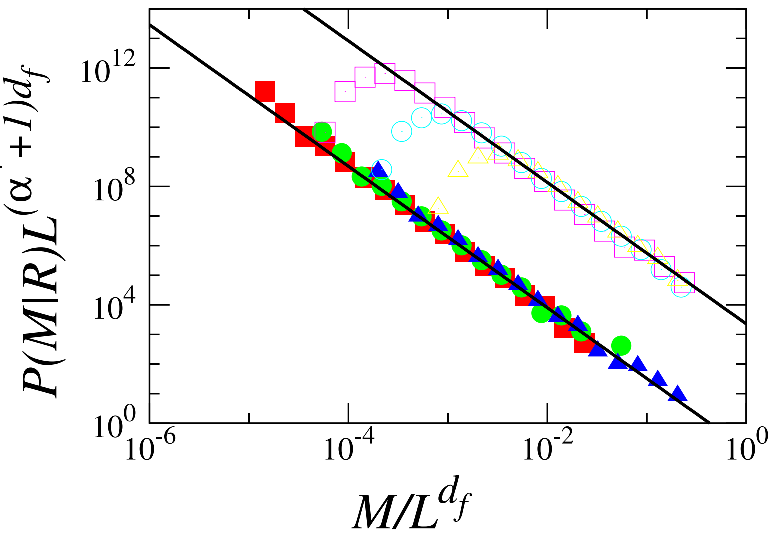


Figure SM3: (color online) Data collapse of $P(M|R)$ for outlet distances $R = 1$ and 10 (filled and open symbols, respectively) for three different system sizes, $L = 129, 257, 513$ (triangles, circles, square, respectively). The solid lines correspond to the power-law, $P(M|R) \propto R^{-(\alpha^*+1)}$, where $\alpha^* = 1.39$ is the exponent for subcritical point-to-point invasion percolation model.
